# Supplementary material for: The effect of source disclosure on evaluation of AI-generated messages: A two-part study
Source: arXiv:2311.15544 ancillary file (2023-11-28)
Supplement: Supplementary file 1 [file Source_Effects_Appendix.pdf]

## Appendix A. Message Generation and Selection Protocol

See Figure A.1 below for a concept illustration of this procedure.

*Collection and Selection of Human Generated Messages*

To create messages comparable to the most retweeted human-generated tweets used in the human evaluation process, we decided to develop prompts for AI message generation based on scraped tweets. Specifically, we used the snscrape package (JustAnotherArchivist, 2021) in Python to collect tweets with #dontvape, #novaping, #quitvaping, #stopvaping, #vapingkills, and #vapingprevention (no date constraints). Using Python code, the individual scraped files were combined, yielding a base corpus of 6,749 raw messages. After exporting the raw messages into a CSV-file, we sorted the tweets by retweet count and used the following criteria to filter the tweets: 1) retweet count of at least 1, 2) English language, 3) non-duplicates, 4) non-advertisement, and 5) longer than 30 characters. The filter processing left 1,384 raw tweets. The raw tweets were further cleaned to remove symbols and white space and saved into a CSV file.

Once we saved the CSV file, we selected 15 most retweeted anti-vaping tweets. We started from the top of the cleaned file, which was already sorted by retweet count, and excluded the tweet if it included one of the following exclusion criteria: 1) did not provide specific information about vaping or the effects of vaping (e.g., "These products are ever-changing and easily hidden by students…"); 2) advertised specific education programs or promoted political policies (e.g., "City of Santa Cruz, in a preliminary vote, supported a ban on flavored tobacco. The second and final vote is coming up in January. #GenerationToEndSmoking #VapingPrevention #YouthInAction"); 3) discussed tobacco without discussing vaping (e.g., "Tobacco use is the leading cause of preventable disease and death in the United States. Nearly all #tobacco use begins during youth and young adulthood. Read more about the latest findings: #SayNoToTobacco #stopvaping"); 4) included possible misinformation (e.g., bc vaping makes you shorter. #scientificallyproven #stopvaping). The selection process ended when we selected 15 tweets. Finally, we cleaned the 15 tweets by removing the hashtags and non-vaping relevant expressions (e.g., "Absolutely!" or "A preclinical study from the University of South Florida has found…"). We took the final steps to remove obvious Twitter cues.

*AI-Message Generation and Selection*

*Prompt-Engineering*

After loading Bloom to Google Colab via the transformer Python package, we conducted the prompt-engineering process. Starting from the most retweeted message, the beginning phrases of each of the tweets were inputted into the Bloom model. Then we evaluated 10 generated tweets for quality. The prompts were discarded if we observed the following red flags: too many of the same messages without much informative content, too many names of official organizations or countries, or clearly false information. A total of 5 prompts were selected for message generation: "Nicotine in vapes", "Vaping is risky", "Vapes and e-cigarettes increase your risk", "Vaping is anything but harmless", and "The substances in e-cigarettes and their vapor include".

*Message Generation and Selection*

Then we generated 100 messages for each of the five prompts with the same set of parameters: max_new_tokens = 60, do_sampling = TRUE, temperature = 0.7, top_k = 40, and top-p = 0.9. Max_new_tokens =60 instructed the model to generate a maximum of 60 additional tokens in length (approximately 45 words). This roughly matched the character limit of Twitter messages. The parameter setting do_sample=True instructed the model to use the sampling approach, or randomly select the next word. The next set of parameters, then, provided the model with details on how to randomly select. The temperature, or the allowed randomness in the text generation, was set to 0.7, aligning with the recommended levels for generating multiple texts (Misri, 2021). Finally, top_k=40 limits the sampling pool of words to 40 words with the highest conditional probability, and top_p=0.9 further limits the pool to the minimum number of words from the 40 that exceed the cumulative probability of 0.9 (von Platen, 2020).

From each of the 100 generated messages, we randomly selected 3 messages, compiling 15 total AI-generated messages to compare to the most retweeted messages. Specifically, we used the random number generator to gather 10 messages per prompt. Then we filtered the messages based on the following exclusion criteria: 1) Included names of official organizations; 2) repetitive information within the sentences; 3) did not advocate against vaping; 4) false information or reference to unverifiable sources. We further cleaned the messages by deleting incomplete ends of the texts and fixed non-natural symbols (e.g., "Äô" for ').

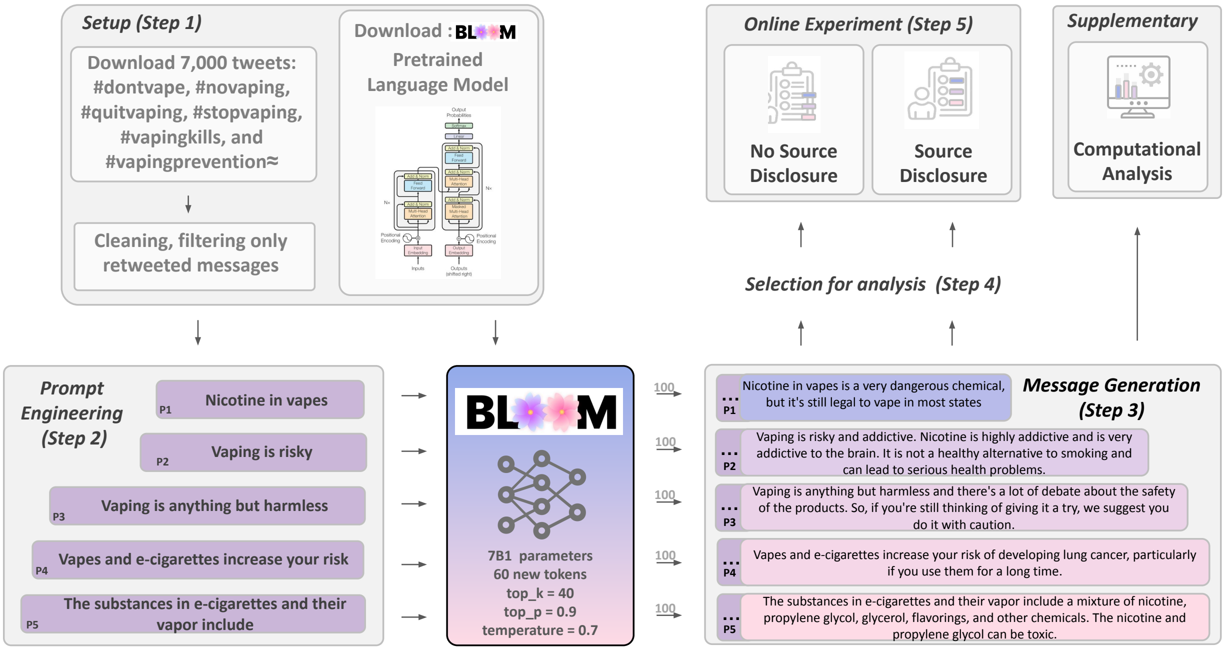


Figure A.1: Conceptual Illustration of AI-message generation.

## Appendix B. Results from Computational Analyses

The results from the computational analysis showed that AI-generated and human-generated messages were similar in terms of semantic structure as well as readability; see Figure B.1). First, semantic analysis of the 30 messages (15 AI and 15 human) used in the experiment via the sentence-transformer package showed that the 30 messages were generally similar, with an average score of .56. Also, the AI-generated messages exhibited greater similarity to each other compared to similarities within the tweets ($m_{similarityAI}$ = .67, $m_{similarityhuman}$ = .47; $p < .001$). Readability analysis showed that both AI-generated messages and human-generated tweets ($m_{Flesch-ScoreAI}$ = 73.2, $m_{Flesch-Scorehuman}$ = 74.4, $p > .05$) were easy to understand (Flesch, 1946).

On the other hand, we found that the content-related features (i.e., word distributions, specific topics discussed, sentiment) differed. The uni- and bi-grams show that AI-generated messages contained more rewards related to the harmful content and effects of vaping (e.g., nicotine, lung cancer, etc.), whereas the tweets included more general statements related to getting help or quitting vaping. Topic modeling provided further support for the topic differences between the two sets of messages - There was more evidence of discussion of topics related to the negative effects of vaping on physical health as well as various components contained in vaping among AI-generated messages. This content aligned more with some of the recommended practices of vaping prevention messages, especially those targeting adolescents and young adults (Boynton et al., 2023; Villanti et al., 2021). Finally, a sentiment analysis using the valence-aware dictionary approach (VADER) showed that AI-generated messages, on average, significantly consisted of more negative sentiment than the human-generated tweets ($m_{FVaderCompoundAI}$ = -.20, $m_{FVaderCompoundhuman}$ = .09, $t$ = 10.37, $p < .001$).

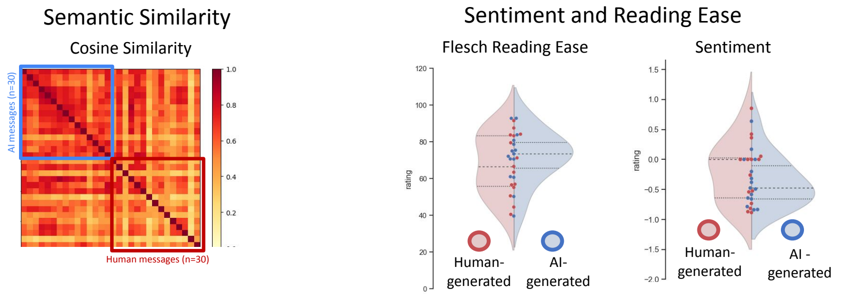


Uni- and Bigram Analysis

| | Human (1,384) | | AI (500) | |
|---|---|---|---|---|
| | *Unigram* | # | *Unigram* | # |
| 1 | vaping | 740 | nicotine | 336 |
| 2 | quitsmoking | 220 | ecigarettes | 234 |
| 3 | quit | 200 | vaping | 230 |
| 4 | help | 178 | lung | 212 |
| 5 | smoking | 170 | cancer | 208 |

| | Human (1,384) | | AI (500) | |
|---|---|---|---|---|
| | *Bigram* | # | *Bigram* | # |
| 1 | smoking vaping | 460 | lung cancer | 112 |
| 2 | stop vaping | 37 | propylene glycol | 92 |
| 3 | quit vaping | 34 | nicotine propylene | 72 |
| 4 | dangers vaping | 32 | glycol glycerin | 66 |
| 5 | quit smoking | 30 | heart disease | 64 |

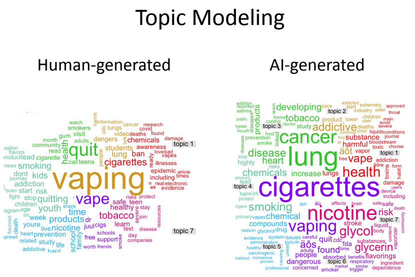


Figure B.2: Conceptual Illustration of AI-message generation.

## References


Boynton, M., Sanzo, N., Brothers, W., Kresovich, A., Sutfin, E., Sheeran, P., Noar, S., 2023. Perceived effectiveness of objective elements of vaping prevention messages among adolescents. Tobacco Control 32, e228–e235.

Flesch, R., 1946. The Art of Plain Talk. Harper and Row, New York, NY.

JustAnotherArchivist, 2021. snscrape: A social networking service scraper in python. Github. URL: https://github.com/JustAnotherArchivist/snscrape.

Misri, I., 2021. How to set sampling temperature for gpt models.

von Platen, P., 2020. How to generate with hugging face. https://huggingface.co/blog/how-to-generate.

Villanti, A.C., LePine, S.E., West, J.C., Cruz, T.B., Stevens, E.M., Tetreault, H.J., Mays, D., 2021. Identifying message content to reduce vaping: Results from online message testing trials in young adult tobacco users. Addictive Behaviors 115, 106778.
